# Supplementary material for: Liquid ropes: a geometrical model for thin viscous jets instabilities
Source: arXiv:1410.5382 ancillary file (2014-10-20)
Supplement: Supplementary file 1 [file si_gm.pdf]

# Supplemental material for ‘Liquid ropes: a geometrical model for thin viscous jets instabilities’

P.-T. Brun, B. Audoly, N. M. Ribe, T. S. Eaves, J. R. Lister

October 20, 2014

## 1 A formula fitting the curvature obtained in numerical simulations of translated coiling

We present a detailed derivation of the empirical fitting law that we introduced in Eq. (2) of the main text.

We first collected numerical data by running the Discrete Viscous Rod method (DVR) over a range of parameters where the translated coiling pattern is observed ($H = 0.6$ and $0 < V/U_c < 0.4$). This pattern was chosen as it sweeps a significant region in the parameter space ($r$,$\phi$). The particular choice of the parameter value $H = 0.6$ is expected to have little influence on the final result as explained further down.

We recorded a time series for the quantities $(r, \phi, \kappa)$ which are defined in figure 3 of the main text: $r$ is the distance of the point of contact with the belt to the vertical projection $O$ of the nozzle onto the belt, $\phi$ is the angle between radial direction (from $O$ to the point of contact) and the tangent to the thread, and $\kappa$ is the curvature of the projection of the thread's centerline onto the plane of the belt at the point of contact. We then used the value of the coiling radius $R_c$ relevant to the height $H = 0.6$ to nondimensionalize $r$ and $\kappa$. The rescaled radius and curvature are defined by

$$\overline{r} = \frac{r}{R_c} \quad \overline{\kappa} = \kappa\, R_c. \tag{1}$$

A fitting law $\overline{\kappa}(\overline{r}, \phi)$ for the numerical data $(\overline{r}, \phi, \overline{\kappa})$ was obtained as follows. We observed that the isolines of the quantity $\phi$ are very close to straight lines when plotted in the plane $\left(\overline{r}, \frac{\overline{\kappa}}{\sqrt{\overline{r}}}\right)$, see figure 1. For any target value of $\phi$, we collected the numerical samples $(\overline{\kappa}, \overline{r})$ whose corresponding $\phi$ matches the target $\phi$ up to a small error $\epsilon \ll 1$, and made a linear fit for $\frac{\overline{\kappa}}{\sqrt{\overline{r}}}$ as a function of $\overline{r}$:

$$\frac{\overline{\kappa}}{\sqrt{\overline{r}}} \approx C(\phi)\,\overline{r} + B(\phi) \quad \text{(best linear fit for fixed } \phi). \tag{2}$$

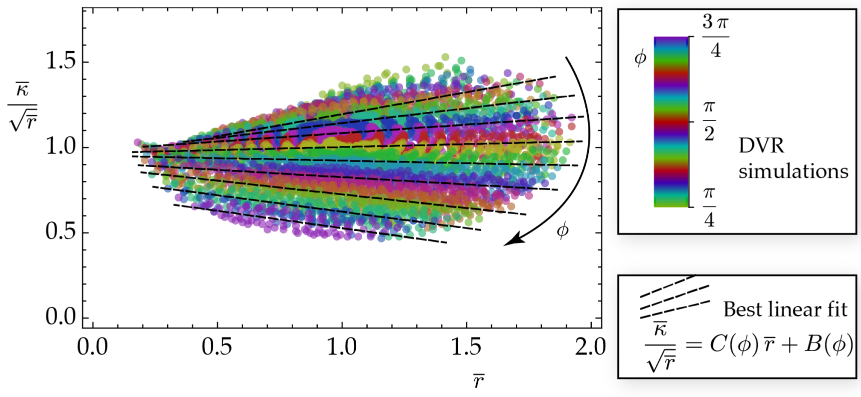


Figure 1: Simulation data for translated coiling from DVR, showing isolines for $\phi$ (coloring) in the $\left(\overline{r}, \frac{\overline{\kappa}}{\sqrt{\overline{r}}}\right)$ plane.

These linear fits correspond to the dashed lines shown in figure 1 (not all the fits are shown in the figure for the sake of legibility).

In figure 2, we show that the constant term in the fitting law in Eq. (2) is very well approximated by a sine function with no adjustable parameter,

$$B(\phi) \approx \sin\phi. \tag{3}$$

The choice of the sine function is compatible with the symmetries of the system. Indeed, in the absence of inertia the viscous hanging thread is invariant by a mirror symmetry with respect to the vertical plane $(Orz)$ containing the nozzle and the point of contact. As a result, $\overline{\kappa}(\overline{r}, \theta)$ is an odd function of $\theta$, and so are $B(\phi)$ and $C(\phi)$. Note that both the original data $(\phi, B(\phi))$ (red dots) and the *symmetrized* data $(-\phi, -B(\phi))$ (blue dots) are fitted in figure 2.

Combining the previous fits, we find

$$\overline{\kappa} \approx \sqrt{\overline{r}}\,\left(1 + A(\phi)\,\overline{r}\right)\,\sin\phi. \tag{4}$$

The fitting function $A(\phi) = \frac{C(\phi)}{B(\phi)}$ is found as follows. We plot the numerical data from DVR in the plane $\left(\phi, \frac{1}{\overline{r}}\left(\frac{\overline{\kappa}}{\sqrt{\overline{r}}\,\sin\phi} - 1\right)\right)$, as shown in figure 3. Note that $\frac{1}{\overline{r}}\left(\frac{\overline{\kappa}}{\sqrt{\overline{r}}\,\sin\phi} - 1\right)$ is the value of $A(\phi)$ predicted by equation (4). The collapse of the simulation data onto a master curve confirms our previous fits. In view of the fact that $A(\phi)$ is an even function, we fit both the original cloud of points coming from the DVR simulation, and the set obtained by mirror symmetry with respect to the vertical axis ($\phi \to -\phi$ symmetry).

We used a fitting function having a single adjustable parameter $b$:

$$A_b(\phi) = \frac{b^2\cos\phi}{1 - b\cos\phi}. \tag{5}$$

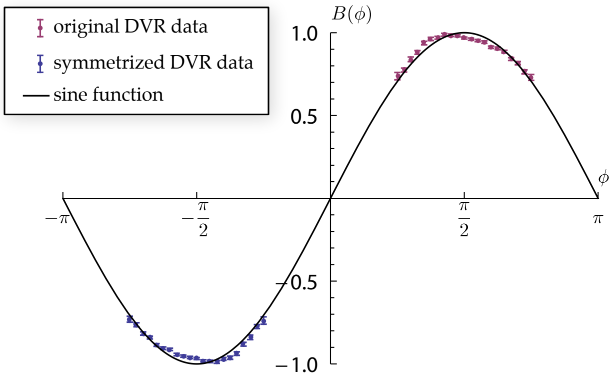


Figure 2: Fit of the constant coefficient $B(\phi)$ by a sine function.

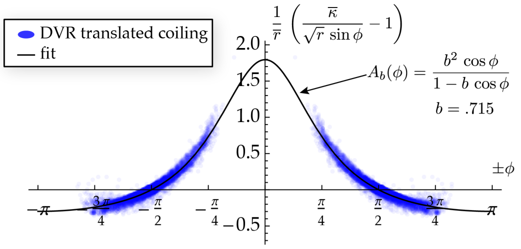


Figure 3: Fitting the quantity $A(\phi)$ in equation (4).

This choice is consistent with the fact that $A(\phi)$ is an even function.

It is also consistent with the existence of the steadily coiling solution, as we now show. In our units, the steadily coiling solution corresponds to $(\overline{r}, \phi, \overline{\kappa}) = (1, \pm\pi/2, 1)$: inserting this into equation (4) yields $A(\pm\pi/2) = 0$. In figure 3, the cloud of numerical data indeed passes through the points $(\pm\pi/2, 0)$. Our fitting functions $A_b(\phi)$ in equation (5) are such that $A(\pm\pi/2) = 0$ for any value of the fitting parameter $b$, as required by the existence of a steadily coiling solution.

The optimal value of the fitting parameter $b$ was found to be

$$b = 0.715 \tag{6}$$

This provides a good fit through the numerical data, as shown in figure 3.

The empirical law for $\overline{\kappa}$ in equations (4–6) has been obtained by fitting numerical data for the *translated coiling pattern* coming from a very small region of the phase diagram (darker vertical red bar in the lower left corner of figure 1b). In the main text, we show that a geometrical model based on this law explains the entire phase diagram.

The entire fitting procedure has been repeated for different values of $H$. For all of them, the curvature was found to be well fitted by equation (4). The optimal value of the parameter $b$ varied within 5%.
